# Supplementary material for: Ferrofluid drop impacts and Rosensweig peak formation in a non-uniform magnetic field
Source: arXiv:2204.05523 source file (2022-04-12)
Supplement: Supplementary file 1 [file supplementary_information.tex]

\newpage

\setcounter{page}{2}
\setcounter{figure}{0}
\setcounter{section}{0}
\setcounter{equation}{0}

\section*{Supplemental Material}

\subsection{Experimental Videos}

High-speed videos for droplets A-D presented in Fig.~\ref{fig:drop_video} are included as Supplemental Material. Each movie has been slowed down 200 times (i.e. captured at 2000 fps and played back at 10 fps). 

\subsection{Comparison of Dimensionless Numbers}

\begin{figure}[ht]
    \centering
    \includegraphics[width=\textwidth]{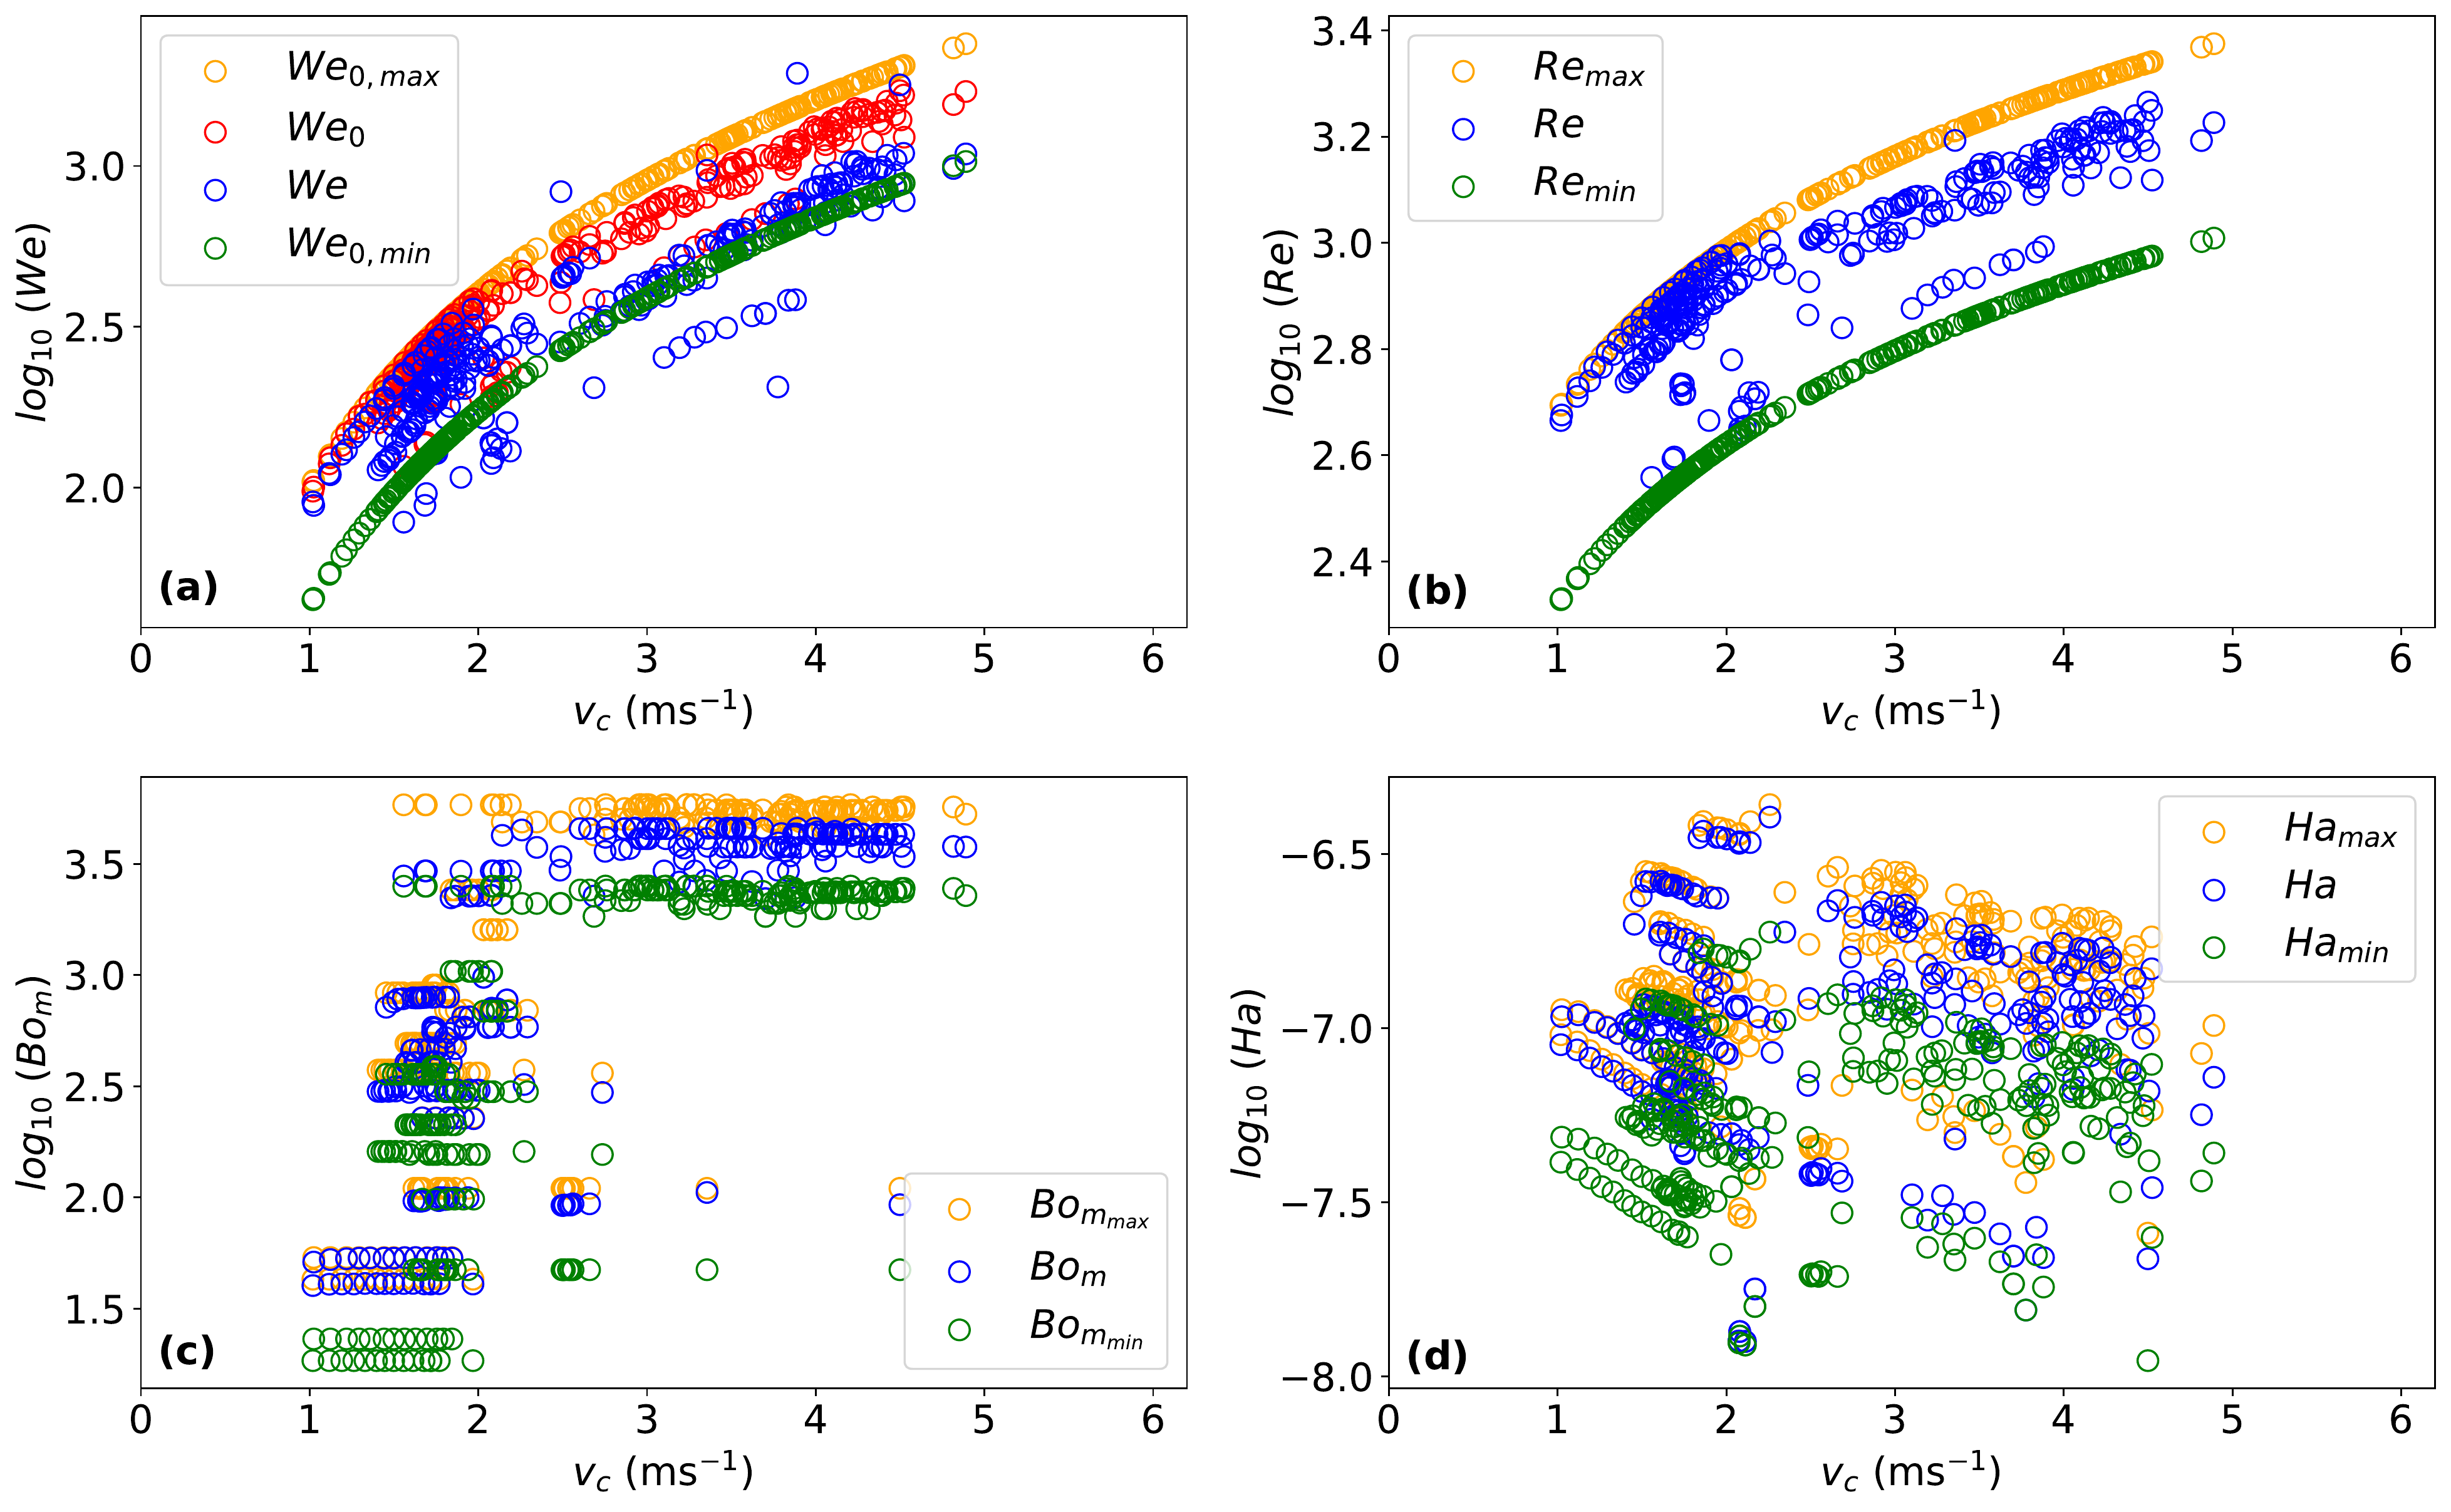}
    \caption{Plots of the dimensionless numbers (a) $We$ and $We_0$, (b) $Re$, (c) $Bo_m$, and (d) $Ha$ as a function of center-of-mass velocity prior to impact. Each plot shows the calculations for each experiment using the three different diameters $D_{max}$, $D_0$, and $D_{min}$ as a length scale.}
    \label{fig:dimensionless}
\end{figure}

A comparison of dimensionless numbers as a function of the centre-of-mass velocity of droplets prior to impact ($v_c$) is presented in Fig.~\ref{fig:dimensionless}. For each of the dimensionless numbers $We_0$, $Re$, $Bo_m$ and $Ha$, values were calculated for each droplet using the equivalent volume $D_0$, as well as bounding values using the smallest ($D_{min}$) and largest ($D_{max}$) equivalent diameters from the data set.

The main dimensionless number used in this work, i.e. values of $We$ from equation (\ref{eqn:We_first_principles}), are included in Fig.~\ref{fig:dimensionless}(a). The difference between $We$ and $We_0$ is caused by drop elongation. Each of $We$, $We_0$ and $Re$ are near-monotonic with respect to $v_c$, although not entirely so due to variable drop size and shape at impact (captured by these numbers). In contrast, $Bo_m$ and $Ha$ are clearly non-monotonic because the impact velocity depends on the applied field.

% \twocolumngrid

\subsection{Measurement of Contact Line Width}

During the initial spread of the droplets, the contact angle is greater than 90\textdegree, so that it is of interest to measure the contact line width as shown in Fig.~\ref{fig:contactline}(a) as well as the drop diameter (i.e. the widest extent of the droplet). The contact line is identified using the clearly visible reflection of the droplet from the glass slide. From a thresholded image of the spreading droplet, a search for concavity on either side (Figure~\ref{fig:contactline}(b)) can be used to identify the edge of the contact line. For analysis, the contact line is defined by a straight line fit through the edge points found on either side of the droplet in 5 different frames. The diameter is similarly found using the central point of concavity at the droplet edge. 

\begin{figure}[ht]
    \centering
    \includegraphics[width=8.6cm]{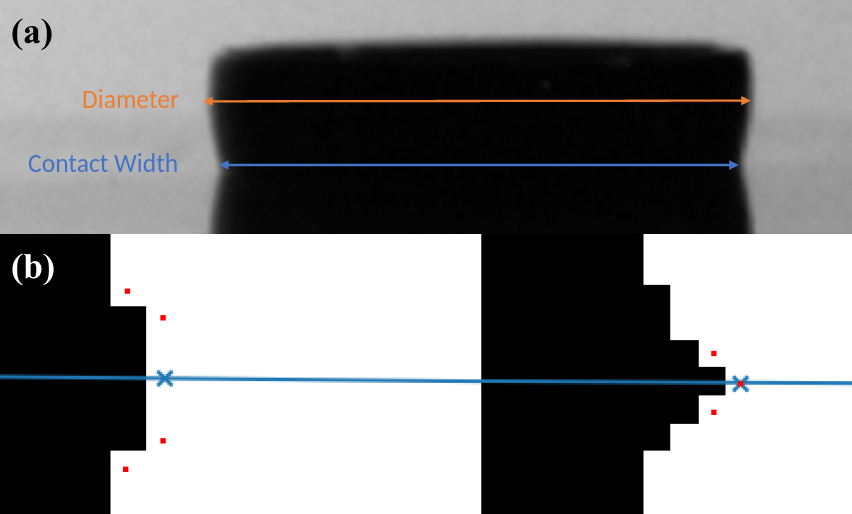}
    \caption{Image analysis for measurement of the contact line width. (a) Image of a ferrofluid drop spreading on a glass slide, with the diameter and contact line width labelled. (b) Magnified image of the left side of a droplet in two different frames (left and right). Individual pixels are visible, and a threshold has been applied so that white pixels represent the imaged droplet, and black pixels represent the background. Red dots define the identified concave contour, the blue crosses indicate contact points, and the blue line is the contact line.}
    \label{fig:contactline}
\end{figure}

\subsection{Maximum Spreading Diameter}

\begin{figure}[ht]
    \centering
    \includegraphics[width=8.6cm]{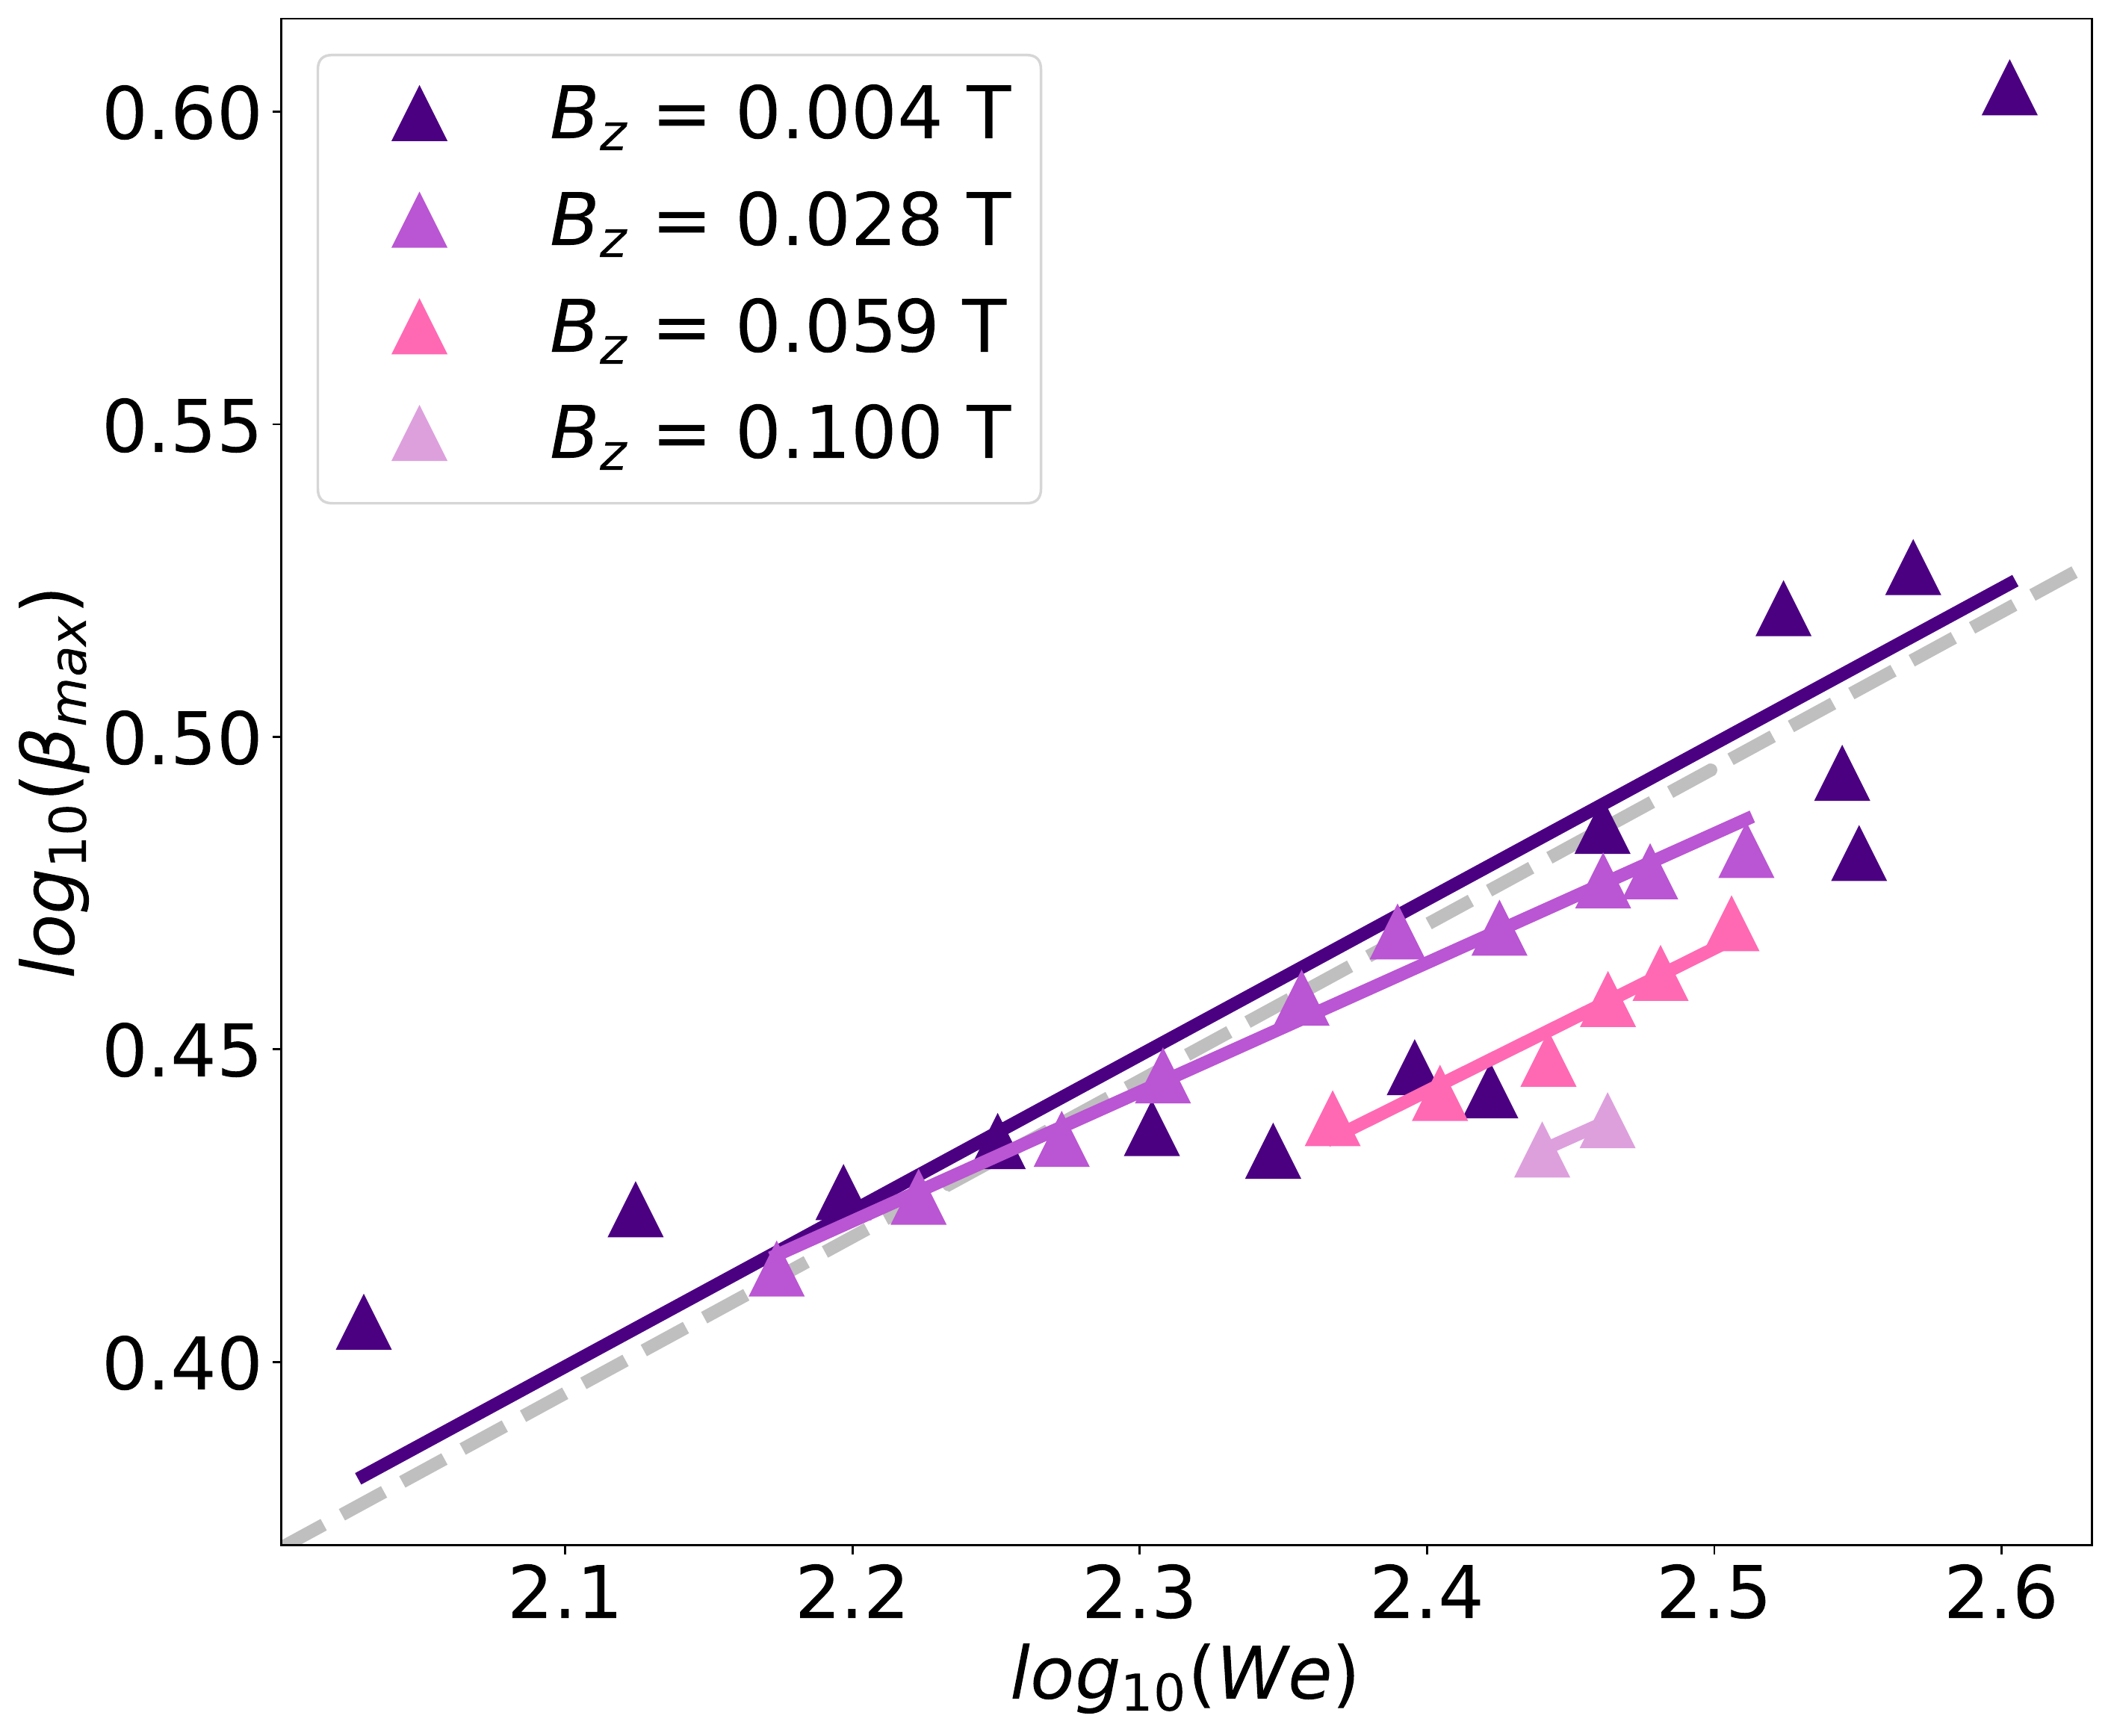}
    \caption{Log-log plot of maximum spread factor as a function of We for a subset of the ferrofluid drop impact experiments with similar droplet size. Solid lines are linear fits to each data set, and the dashed grey line has a gradient of 0.25.}
    \label{fig:max_spread_vs_velocity}
\end{figure}

Figure \ref{fig:max_spread_vs_velocity} shows the relation between the normalized maximum spreading diameter, the impact Weber number, and the $B$-field for experiments conducted at relatively low $B_z$. Low $B_z$ data are appropriate to use because the initial spread of the droplet can be distinguished from more long-term rebound or growth of the spreading diameter. Furthermore, for these data the average volume of the droplets was reasonably constant at $7.29 \pm 0.14~\mu$l. 

As expected, the maximum spread generally increases with $We$ for any particular magnet position. With increasing $B$-field, the maximum spread generally decreases. This is consistent with the increased inwards radial force that the droplets experience for these $B_z$ values (the fields considered here are not sufficient to cause rim formation, see Section \ref{Sec:rim}). Linear fits were calculated and plotted for data points at each value of $B_z$. For droplet impacts on solid surfaces, maximum spread is often observed to scale as $\beta_{\text{max}} \propto \text{We}^{0.25}$ \cite{Marengo}. The fits in Fig.~\ref{fig:max_spread_vs_velocity} all have a gradient close to 0.25 (shown by the dashed grey line) although the data are limited and inconclusive in some places. 

\subsection{Rim Coalescence for Inner Peaks}

\begin{figure}[ht]
    \centering
    \includegraphics[width=8.6cm]{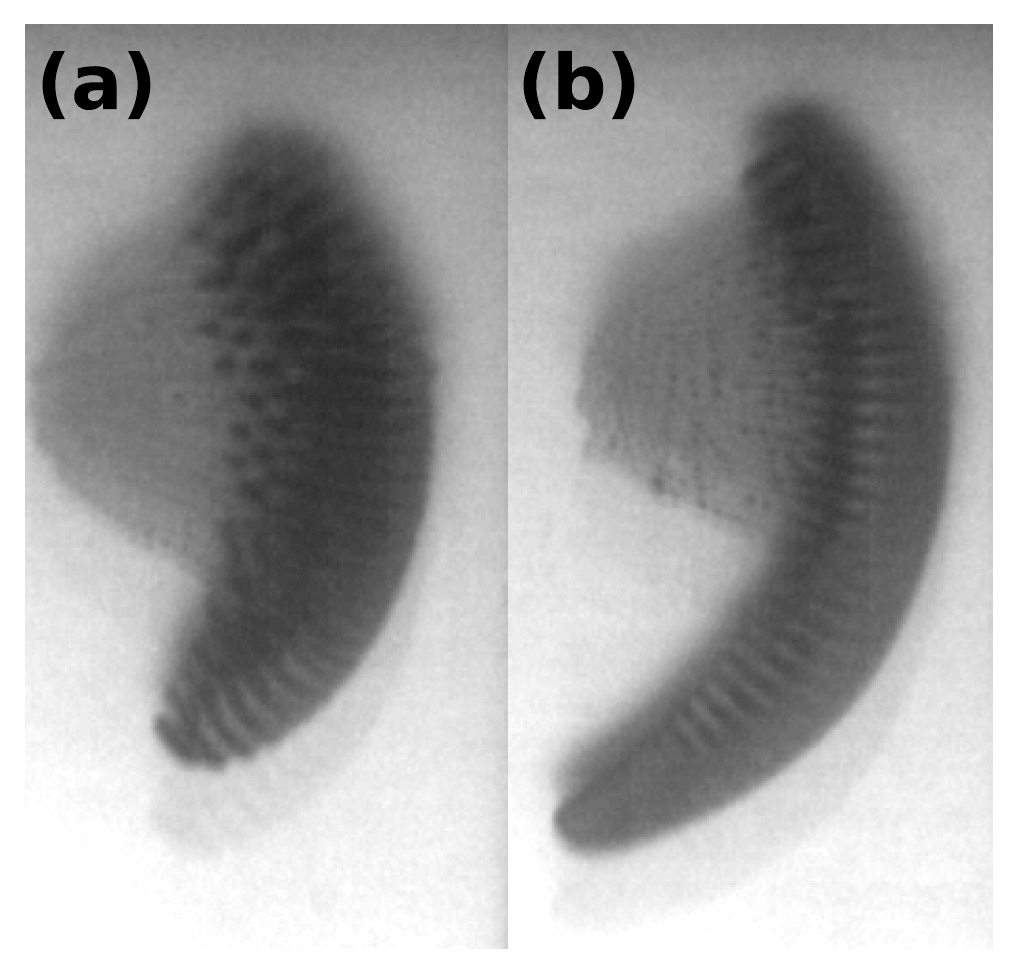}
    \caption{ 
    Images of droplets at 37~s after impact producing slightly different rim morphologies. (a) $We = 393$, $V = 2.54$~$\mu$l, $v = 3.11$~m/s, $h_0 = 3.47$~mm, $B = 0.319$~T. (b) $We = 453$, $V = 2.79$~$\mu$l, $v = 3.23$~m/s, $h_0 = 2.26$~mm, $B = 0.358$~T. 
    }
    \label{fig:rim_other}
\end{figure}

Figure \ref{fig:rim_other} shows two asymmetric rims formed after slightly off-centre impacts at relatively high magnetic field, pictured a long time after impact. In Fig.~\ref{fig:rim_other}(a), peaks on the inner side of the rim have not coalesced with the rim, in contrast with Fig.~\ref{fig:rim_other}(b). In the latter case, the magnetic field strength is higher, suggesting that a relatively high field is required to overcome peak repulsion and produce coalescence with the rim. Also note that the width of the rim is smaller when the field is greater.
